# Supplementary material for: Uncertainty Propagation on Unimodular Matrix Lie Groups
Source: arXiv:2312.03348 source file (2023-12-06)
Supplement: Supplementary file 1 [file appendix1.tex]

In this section, we construct the left and right Jacobian matrix for a matrix Lie group that has been extended through the semi-direct product operation. That is, consider the group $H$ and and $N$ dimensional group $G$ that obey the following relation:
\begin{equation}
    H = G \ltimes \mathbb{R}^N,
\end{equation}
where now $H$ is a $2N$ dimensional group. This is similar to (but more general) than a (co-)tangent bundle extension that was explored in \cite{jayaraman2020black}. We can write an element, $h\in H$ in terms of an element $g\in G$ and a vector $\boldsymbol{v}\in\mathbb{R}^N$ through the homogeneous matrix:
\begin{equation}
h = \left(
    \begin{array}{c|c}
    \Phi(g) & \boldsymbol{v}\\
    \hline
    \boldsymbol{0}^T & 1
    \end{array}\right),
\end{equation}
where $\Phi(g)$ is a faithful matrix representation of $G$. Let $h(\boldsymbol{q},\boldsymbol{v}) = h(g(\boldsymbol{q}),\boldsymbol{v})$ fix the parameterization of $H$. If $J_R(g(\boldsymbol{q}))$ is the right Jacobian for $G$ in this parameterization and $J_L(g(\boldsymbol{q}))$ is the left Jacobian, we have, for $\mathcal{J}_R(\boldsymbol{q},\boldsymbol{v})$ and $\mathcal{J}_L(\boldsymbol{q},\boldsymbol{v})$ representing the right and left Jacobians of $H$:
\begin{equation}\label{eq:GeneralJR}
    \mathcal{J}_R = \left(
    \begin{array}{c|c}
    J_R(\boldsymbol{q}) & \mathbb{O}\\
    \hline
    \mathbb{O} & \Phi^{-1}(g)
    \end{array}\right),
\end{equation}
\begin{equation}\label{eq:GeneralJL}
    \mathcal{J}_L = \left(
    \begin{array}{c|c}
    J_L(\boldsymbol{q}) & \mathbb{O}\\
    \hline
    X(\boldsymbol{q},\boldsymbol{v}) & \mathbb{I}
    \end{array}\right),
\end{equation}
where,
\begin{equation*}
    X = \left[-\left(\frac{\partial \Phi}{\partial q_1}\Phi^{-1}\boldsymbol{v}\right)^\vee,\cdots,-\left(\frac{\partial \Phi}{\partial q_N}\Phi^{-1}\boldsymbol{v}\right)^\vee\right].
\end{equation*}
Then if $E^R$ and $E^L$ denote the Lie derivative operators for the group $G$ and the Lie derivative operators for $H$ are denoted by $\tilde{E}^R$ and $\tilde{E}^L$, we have the following results:
\begin{equation}
    \tilde{E}^R =
    \begin{pmatrix}
    E^R\\
    \Phi^{-1}(g(\boldsymbol{q}))\partial/\partial\boldsymbol{v}
    \end{pmatrix},
\end{equation}
\begin{equation}
    \tilde{E}^L =
    \begin{pmatrix}
    E^L + J^{-T}_L(\boldsymbol{q}) X^T(\boldsymbol{q},\boldsymbol{v})\partial/\partial \boldsymbol{v}\\
    -\partial/\partial\boldsymbol{v}
    \end{pmatrix}.
\end{equation}
It can be seen that upper-right block for $\mathcal{J}_R$ and $\mathcal{J}_L$ is a zero block. This motivates the reasoning in the proof of the second part of Theorem 1.

On the other hand, an element $h'$ that lives in the $2N$ dimensional left-trivialised (co-)tangent bundle group $H'$ (that is extended from an $N$-dimensional group $G$) would have the following matrix representations, 
\begin{equation}
    h' = \left(\begin{array}{c|c}
    \Phi(g) & \boldsymbol{0}\\
    \hline
    \boldsymbol{v}^T & 1
    \end{array}\right),
\end{equation}
where $\phi(g)$ is yet again a faithful matrix representation of $G$. The left-trivialised bundle groups are introduced in \cite{engo2003partitioned}. Let $h'(\boldsymbol{q},\boldsymbol{v}) = h'(g(\boldsymbol{q}),\boldsymbol{v})$ fix the parameterization of $H'$. Then, the right and left Jacobians for $H'$ can be written as,
\begin{equation}
    \mathcal{J}_R' = \left(\begin{array}{c|c}
    J_R(\boldsymbol{q}) & \mathbb{O}\\
    \hline
    X'(\boldsymbol{q},\boldsymbol{v}) & \mathbb{I}
    \end{array}\right),
\end{equation}
\begin{equation}
    \mathcal{J}_L' = \left(\begin{array}{c|c}
    J_L(\boldsymbol{q}) & \mathbb{O}\\
    \hline
    \mathbb{O} & \Phi^{-T}(g)
    \end{array}\right).
\end{equation}
Yet again we see that the upper-right block of the right and left Jacobians is a zero matrix. This suggests that the reasoning in the proof of the second part of Theorem \ref{thm:Thm1} holds for left-trivialised (co-)tangent bundles as well.
