# Supplementary material for: Uncertainty Propagation on Unimodular Matrix Lie Groups
Source: arXiv:2312.03348 source file (2023-12-06)
Supplement: Supplementary file 2 [file appendix2.tex]

% The BCH expansion for $Z = \log(e^Xe^Y)$ is,
% \begin{multline}
%     Z = X + Y + \frac{1}{2}[X,Y] + \frac{1}{12}([X,[X,Y]] + [Y,[Y,X]]) +\\+ \frac{1}{48}([Y,[X,[Y,X]]] + [X,[Y,[Y,X]]]) + \cdots,
% \end{multline}
% where $[X,Y] = XY - YX$ and the subsequent terms involve at least five appearances of $X$ or $Y$ in the recursive Lie brackets (i.e., for instance $[Y,[Y,[Y,[Y,X]]]]$).

% We first see that,
% \begin{multline}\label{eq:BCH_left}
%     [\log^\vee(e^{-tE_i}\circ k)] - [\log^\vee k] = -t\boldsymbol{e}_i - \frac{t}{2}ad_i\boldsymbol{x} -\\- \frac{t}{12}ad_Xad_X\boldsymbol{e}_i + \mathcal{O}(t,||\boldsymbol{x}||^4),
% \end{multline}
% and,
% \begin{multline}\label{eq:BCH_right}
%     [\log^\vee(k \circ e^{tE_i})] - [\log^\vee k] = t\boldsymbol{e}_i - \frac{t}{2}ad_i\boldsymbol{x} +\\+ \frac{t}{12}ad_Xad_X\boldsymbol{e}_i + \mathcal{O}(t,||\boldsymbol{x}||^4).
% \end{multline}

% From here, we can see that,
% \begin{align*}
%     E^L_i\boldsymbol{x} &= \lim_{t\rightarrow 0}\left(\frac{[\log^\vee (e^{-tE_i}\circ k)] - [\log^\vee k]}{t}\right) \\&\approx -\boldsymbol{e}_i - \frac{1}{2}ad_i\boldsymbol{x} - \frac{1}{12}ad_Xad_X\boldsymbol{e}_i + \mathcal{O}(||\boldsymbol{x}||^4),
% \end{align*}
% and,
% \begin{align*}
%     E^R_i\boldsymbol{x} &= \lim_{t\rightarrow 0}\left(\frac{[\log^\vee (k\circ e^{tE_i})] - [\log^\vee k]}{t}\right) \\&\approx \boldsymbol{e}_i - \frac{1}{2}ad_i\boldsymbol{x} + \frac{1}{12}ad_Xad_X\boldsymbol{e}_i + \mathcal{O}(||\boldsymbol{x}||^4).
% \end{align*}

% Therefore, with an error of order $\mathcal{O}(||\boldsymbol{x}||^3)$ we obtain,
% \begin{align}\nonumber
%     E^L_i\left(\boldsymbol{x}\boldsymbol{x}^T\right) &\approx -\boldsymbol{x}\left(\boldsymbol{e}_i + \frac{1}{2}ad_i\boldsymbol{x}\right)^T - \left(\boldsymbol{e}_i + \frac{1}{2}ad_i\boldsymbol{x}\right)\boldsymbol{x}^T\\\label{eq:ELloglog}
%     &\approx -\boldsymbol{x}\boldsymbol{e}^T_i - \boldsymbol{e}_i\boldsymbol{x}^T - \frac{1}{2}\boldsymbol{x}\boldsymbol{x}^Tad_i^T - \frac{1}{2}ad_i\boldsymbol{x}\boldsymbol{x}^T.
% \end{align}
% Similarly we have,
% \begin{equation}\label{eq:ERloglog}
%     E^R_i(\boldsymbol{x}\boldsymbol{x}^T) = \boldsymbol{x}\boldsymbol{e}^T_i + \boldsymbol{e}_i\boldsymbol{x}^T - \frac{1}{2}\boldsymbol{x}\boldsymbol{x}^Tad_i^T - \frac{1}{2}ad_i\boldsymbol{x}\boldsymbol{x}^T.
% \end{equation}

% A term that we will appear is, $E^L_iE^L_j\boldsymbol{x}$, which we can expand with an error of $\mathcal{O}(||\boldsymbol{x}||^3)$ to obtain,
% \begin{multline}\nonumber
%     E^L_iE^L_j\boldsymbol{x} \approx \frac{1}{2}ad_j\left(\boldsymbol{e}_i + \frac{1}{2}ad_i\boldsymbol{x} + \frac{1}{12}ad_Xad_X\boldsymbol{e}_i\right) -\\-  \frac{1}{12}E^L_i(ad_Xad_X)\boldsymbol{e}_j
% \end{multline}
% Since $ad_X$ is linear in $\boldsymbol{x}$, to ensure that  $E^L_iE^L_j\boldsymbol{x}$ has an error of $\mathcal{O}(||\boldsymbol{x}||^3)$, we can truncate the expansion of $E^L_i(ad_X)$ with an error of $\mathcal{O}(||\boldsymbol{x}||^2)$. Similarly,
% \begin{multline}\label{eq:ERiERjlog}
%     E^R_iE^R_j\boldsymbol{x} \approx \frac{1}{2}ad_j\left(\boldsymbol{e}_i - \frac{1}{2}ad_i\boldsymbol{x} + \frac{1}{12}ad_Xad_X\boldsymbol{e}_i\right) +\\+ \frac{1}{12}E^R_i(ad_Xad_X)\boldsymbol{e}_j
% \end{multline}

% The following is true by the product rule:
% \begin{multline*}
% E^L_iE^L_j(\boldsymbol{x}\boldsymbol{x}^T) = (E^L_iE^L_j\boldsymbol{x})\boldsymbol{x}^T + E^L_j\boldsymbol{x}E^L_i\boldsymbol{x}^T +\\+ E^L_i\boldsymbol{x}E^L_j\boldsymbol{x}^T + \boldsymbol{x}(E^L_iE^L_j\boldsymbol{x}^T),
% \end{multline*}
% where the $E^L_i\boldsymbol{x}$ term has to be expanded with an error of $\mathcal{O}(||\boldsymbol{x}||^3)$ but $E^L_iE^L_j\boldsymbol{x}$ only needs to have an error of $\mathcal{O}(||\boldsymbol{x}||^2)$ in the expressions in the paper (since it is usually multiplied with another quantity of order $\mathcal{O}(||\boldsymbol{x}||)$). Likewise,
% \begin{multline*}
% E^R_iE^R_j(\boldsymbol{x}\boldsymbol{x}^T) = (E^R_iE^R_j\boldsymbol{x})\boldsymbol{x}^T + E^R_j\boldsymbol{x}E^R_i\boldsymbol{x}^T +\\+ E^R_i\boldsymbol{x}E^R_j\boldsymbol{x}^T + \boldsymbol{x}(E^R_iE^R_j\boldsymbol{x}^T),
% \end{multline*}

% The previous two expressions rely on knowing $E^L_iad_X$ and $E^R_iad_X$ with an error of at most $\mathcal{O}(||\boldsymbol{x}||^2)$. We first note that,
% \begin{equation}
%     ad(c_1X + c_2Y) = c_1ad(X) + c_2ad(Y),
% \end{equation}
% by linearity for two constants $c_1$ and $c_2$. This can also be seen by assuming an arbitrary $Z$ such that $ad(c_1X + c_2Y)Z = [c_1X+c_2Y,Z] = c_1[X,Z] + c_2[Y,Z] = c_1ad(X)Z + c_2ad(Y)Z = (c_1ad(X) + c_2ad(Y))Z$. Since this holds for any $Z$, the above identity follows. Then,
% \begin{align}\nonumber
%     E^L_i(ad_X) &= \lim_{t\rightarrow 0}\left(\frac{[ad(\log(e^{-tE_i}\circ k))] - [ad(\log k)]}{t}\right) \\&\approx 
%     -ad_i - \frac{1}{2}ad_{[E_i,X]},
% \end{align}
% and,
% \begin{align}\nonumber
%     E^R_i(ad_X) &= \lim_{t\rightarrow 0}\left(\frac{[ad(\log(k\circ e^{tE_i}))] - [ad(\log k)]}{t}\right) \\&\approx 
%     ad_i - \frac{1}{2}ad_{[E_i,X]}.
% \end{align}
% Using these results we have, to an error of $\mathcal{O}(||\boldsymbol{x}||^3)$,
% \begin{multline}\label{eq:ELiEljlog}
%     E^L_iE^L_j\boldsymbol{x} \approx \frac{1}{2}ad_j\boldsymbol{e}_i + \frac{1}{4}ad_jad_i\boldsymbol{x} +\\+ \frac{1}{24}ad_jad_Xad_X\boldsymbol{e}_i + \frac{1}{12}\left(ad_iad_X\boldsymbol{e}_j + ad_Xad_i\boldsymbol{e}_j\right)+\\+ \frac{1}{24}\left(ad_{[E_i,X]}ad_X\boldsymbol{e}_j + ad_Xad_{[E_i,X]}\boldsymbol{e}_j\right),
% \end{multline}
% and if we define $P$ and $S$ as the following collection of terms:
% \begin{multline*}
%     P = \frac{1}{2}ad_j\boldsymbol{e}_i\boldsymbol{x}^T + \frac{1}{4}ad_jad_i\boldsymbol{x}\boldsymbol{x}^T +\\+\frac{1}{12}\left(ad_iad_X\boldsymbol{e}_j\boldsymbol{x}^T + ad_Xad_i\boldsymbol{e}_j\boldsymbol{x}^T\right),
% \end{multline*}
% \begin{multline*}
%     S = \boldsymbol{e}_i\boldsymbol{e}_j^T + \frac{1}{2}\left(\boldsymbol{e}_i\boldsymbol{x}^Tad_j^T + ad_i\boldsymbol{x}\boldsymbol{e}_j^T\right) +\\+ \frac{1}{4}ad_i\boldsymbol{x}\boldsymbol{x}^Tad_j^T + \frac{1}{12}\left(\boldsymbol{e}_i\boldsymbol{e}_j^Tad_X^Tad_X^T + ad_Xad_X\boldsymbol{e}_i\boldsymbol{e}^T_j\right),
% \end{multline*}
% we would have,
% \begin{equation}\label{eq:ELiEljloglog}
%     E^L_iE^L_j(\boldsymbol{x}\boldsymbol{x}^T) \approx P + P^T + S + S^T
% \end{equation}


% When we have a distribution $f(g)$ on a matrix Lie group $G$, we can define the (right) mean $\mu_r$ and covariance $\Sigma_r$ as the definition \ref{def:r_mean_cov}.
% It is also possible to define the left mean $\mu_l$ and covariance $\Sigma_l$ as,
% \begin{equation}
%     \int_G \log^{\vee}(\mu_l^{-1}\circ g)f(g)dg\doteq \boldsymbol{0},
% \end{equation}
% and,
% \begin{equation}
%     \Sigma_l \doteq \int_G [\log^{\vee}(\mu_l^{-1}\circ g)][\log^{\vee}(\mu_l^{-1}\circ g)]^T f(g)dg.
% \end{equation}
% These two definitions are in fact correlated.
% Before introducing the correlation, we need to define the adjoint representation of a Lie group:
% \begin{definition}
%     The adjoint operator $Ad:G\rightarrow GL(\mathcal{G})$ of a matrix Lie group $G$ is defined by the following equation:
%     \begin{equation}
%         Ad(g)X\doteq gXg^{-1}.
%     \end{equation}
% \end{definition}
% When we write an element $X$ of the Lie algebra $\mathcal{G}$ as a vector $\boldsymbol{x}=X^{\vee}$, the adjoint operator is a matrix $[Ad(g)]$ and we have $[Ad(g)]X^{\vee}=(Ad(g)X)^{\vee}$.
% The formula for $[Ad(g)]$ is:
% \begin{equation}
%     [Ad(g)]=[(gE_1 g^{-1})^{\vee}, \,(gE_2 g^{-1})^{\vee},\,...,\,(gE_N g^{-1})^{\vee}].
% \end{equation}
% The following property of $Ad(g)$ is useful:
% \begin{equation} \label{eq:Ad_property}
%     Ad(g_1)\log(g_2)=\log(g_1 g_2  g_1^{-1}).
% \end{equation}
% It comes directly from the property of the exponential of a matrix:
% \begin{equation*}
%     \exp\left(g_1  \log(g_2)  g_1^{-1}\right)=g_1\exp\left(\log(g_2)\right) g_1^{-1}=g_1 g_2  g_1^{-1}.
% \end{equation*}

% The following theorem states the relationship between two types of definitions of mean and covariance:
% \begin{theorem}
%     The left mean equals the right mean of a distribution:
%     \begin{equation}
%         \mu\doteq \mu_l = \mu_r.
%     \end{equation}
%     The left and right covariances are related by:
%         \begin{equation}
%             \Sigma_l = [Ad(\mu)]^{-1}\Sigma_r [Ad(\mu)]^{-T}.
%         \end{equation}
%     \begin{proof}
%     Using the property of $Ad(g)$, Eq. (\ref{eq:Ad_property}), we have,
%     \begin{equation*}
%     \begin{aligned}
%         \log^{\vee}(\mu^{-1}\circ g)&=\log^{\vee}\left( \mu^{-1}\circ (g\circ \mu^{-1})\circ \mu \right)\\
%         &=[Ad(\mu^{-1})]\log^{\vee}(g\circ \mu^{-1}).
%     \end{aligned}
%     \end{equation*}
%     Substituting the equation into the definition of (left) mean and covariance directly yields the result.
%     \end{proof}
% \end{theorem}
